# Supplementary material for: Untangling Dense Non-Planar Knots by Learning Manipulation Features and Recovery Policies
Source: arXiv:2107.08942 source file (2021-06-29)
Supplement: Supplementary file 1 [file 9-appendix.tex]

\section{Appendix}

\subsection{LOKI}
\subsubsection{Simulator Details}
\subsubsection{Training Details}

\subsection{SPiDERMan}
We train SPiDERMan's learned density-comparison perception component on 350 pairs of images and employ data augmentation techniques according to Table~\todo{data aug table}

\subsection{Experimental Details}
